# Supplementary material for: iMatching: Imperative Correspondence Learning
Source: arXiv:2312.02141 source file (2025-01-28)
Supplement: Supplementary file 1 [file main_supp.tex]

\documentclass[runningheads]{llncs}

% ---------------------------------------------------------------
% Include basic ECCV package
 
\usepackage{eccv}

% OPTIONAL: Un-comment the following line for a version which is easier to read
% on small portrait-orientation screens (e.g., mobile phones, or beside other windows)
%\usepackage[mobile]{eccv}

% ---------------------------------------------------------------
% Other packages

% Commonly used abbreviations (\eg, \ie, \etc, \cf, \etal, etc.)
\usepackage{eccvabbrv}

% Include other packages here, before hyperref.
\usepackage{graphicx}
\usepackage{booktabs}
\usepackage[free-standing-units=true]{siunitx}

% The "axessiblity" package can be found at: https://ctan.org/pkg/axessibility?lang=en
\usepackage[accsupp]{axessibility}  % Improves PDF readability for those with disabilities.

% ---------------------------------------------------------------
% Hyperref package

% It is strongly recommended to use hyperref, especially for the review version.
% Please disable hyperref *only* if you encounter grave issues.
% hyperref with option pagebackref eases the reviewers' job, but should be disabled for the final version.
%
% If you comment hyperref and then uncomment it, you should delete
% main.aux before re-running LaTeX.
% (Or just hit 'q' on the first LaTeX run, let it finish, and you
%  should be clear).

\usepackage{hyperref}

% Support for ORCID icon
\usepackage{orcidlink}

% custom packages
\usepackage{physics}
\usepackage{tabularx}
\usepackage[normalem]{ulem}
\usepackage{colortbl}
\usepackage[super]{nth}
\usepackage{wrapfig}
\setlength{\belowcaptionskip}{0pt plus 0pt minus 0pt}
\usepackage{footnote}

\let\llncssubparagraph\subparagraph
%% Provide a definition to \subparagraph to keep titlesec happy
\let\subparagraph\paragraph
%% Load titlesec
\usepackage[compact]{titlesec}
%% Revert \subparagraph to the llncs definition
\let\subparagraph\llncssubparagraph
\titlespacing{\section}{0pt}{2ex}{1ex}
\titlespacing{\subsection}{0pt}{1ex}{0.2ex}
\titlespacing{\subsubsection}{0pt}{0.3ex}{0.1ex}
% \captionsetup{belowskip=-15pt}
% \captionsetup{aboveskip=5pt}

\hypersetup{
  hidelinks
}

%%%%%%%%% ds new commands

% \usepackage{natbib}

\begin{document}

\renewcommand*{\thefootnote}{\fnsymbol{footnote}}
\footnotetext[1]{Equal contribution.}
\renewcommand*{\thefootnote}{\arabic{footnote}}

\input{supp/6-supp}

\end{document}
